# Supplementary material for: HPNet: Deep Primitive Segmentation Using Hybrid Representations
Source: arXiv:2105.10620 source file (2021-10-21)
Supplement: Supplementary file 1 [file 07_supp.tex]

\section{Supplementary Material}
\subsection{Additional Analysis of the Spectral Embedding Module}

This section provides a proof on the following result of the main paper, which states that when $n_k = \frac{n}{K}$,
\begin{equation}
\min\limits_{R\in O(K)}\frac{\|U_{\cons}R-U_{\cons}^{\good}\|_{\set{F}}}{\|U_{\cons}^{\good}\|_{\set{F}}} = O\left({\scriptstyle \frac{2K\sqrt{\rho}}{(1-\rho)+\sqrt{1-\rho}}} n^{-\frac{1}{4}}\right).
\label{Eq:Spectral:Embedding:Error}
\end{equation}

To obtain this result, we first look at $E$. It is clear that if the prediction associated with a point is incorrect, then it would affect $O(\sqrt{n})$ edges. Therefore,
\begin{equation}
\|E\|_{\set{F}} \in O\left(\sqrt{\rho}n^{\frac{3}{4}}\right).
\label{Eq:Error}
\end{equation}
 
Likewise, if the shape prediction associated with a point is correct, it will introduce edges for each point within the same primitive. Suppose the size of each primitive is $n_k$ and the number of correct predictions $(1-\rho)n_k$. We proceed to characterize the spectrum of $A_{\cons,k}^{\good}$.
\begin{proposition}
The eigenvalues of $A_{\cons,k}^{\good}$ are given by
\begin{equation}
\lambda_i(A_{\cons,k}^{\good}) = 
%\left\{
%\begin{array}{cc}
%n_k\frac{(1-\rho)+\sqrt{1-\rho}}{2} & i = 1 %\\
%0 & 1 < i < n_k \\
%n_k\frac{(1-\rho)-\sqrt{1-\rho}}{2} & i = %n_k
%\end{array}
%\right.\
\begin{cases}
n_k\frac{(1-\rho)+\sqrt{1-\rho}}{2}, & i=1\\
0, & 1 < i < n_k\\
n_k\frac{(1-\rho)-\sqrt{1-\rho}}{2}, & i = n_k.
\end{cases}
\label{Eq:Eigen:Value}
\end{equation}
\label{Prop:1}
\end{proposition}
\noindent\textsl{Proof:} Proof of Section~\ref{Subsec:Prop:1}.

Suppose $n_k = \frac{n}{K}$. We can derive (\ref{Eq:Spectral:Embedding:Error}) by substituting (\ref{Eq:Error}) and (\ref{Eq:Eigen:Value}) into the following variant of the Davis-Kahan theorem which is copied from the main paper:
\begin{equation}
\min\limits_{R\in O(K)}\|U_{\cons}R-U_{\cons}^{\good}\|_{\set{F}} \leq \frac{\sqrt{\lambda_{1}(A_{\cons}^{\good}})\|E\|_{\set{F}}}{\lambda_{K}(A_{\cons}^{\good})-\lambda_{K+1}(A_{\cons}^{\good})}.
\end{equation}

(\ref{Prop:1}) implies when the fractions of wrong shape predictions are small, the spectral gap $\lambda_{K}(A_{\cons,k}^{\good}) - \lambda_{K+1}(A_{\cons,k}^{\good})$ is large, which implies the advantage of using $U_{c}^{\good}$ over the predicted shape parameters for clustering.

\subsubsection{Proof of Prop.~\ref{Prop:1}}
\label{Subsec:Prop:1}

Without losing generality, we assume the correct predictions occupy the first $\rho n_k$ elements. It it easy see to check that 
$$
A_{\cons,k}^{\good} = \left(
\begin{array}{c}
\bs{1} \\
\frac{1}{2}\bs{1}
\end{array}
\right)\left(
\begin{array}{c}
\bs{1} \\
\frac{1}{2}\bs{1}
\end{array}
\right)^T - \frac{1}{4} \left(
\begin{array}{c}
\bs{0} \\
\bs{1}
\end{array}
\right)\left(
\begin{array}{c}
\bs{0} \\
\bs{1}
\end{array}
\right)^T.
$$
Therefore, the rank of $A_{\cons,k}^{\good}$ is $2$. It is easy to check that the two non-zero eigenvalues of $A_{\cons,k}^{\good}$ are 
\begin{align*}
\lambda_1(A_{\cons,k}^{\good}) & = n_k\frac{(1-\rho)+\sqrt{(1-\rho)}}{2} \\ \lambda_{n_k}(A_{\cons,k}^{\good}) & = n_k\frac{(1-\rho)-\sqrt{1-\rho}}{2},
\end{align*}
and the corresponding eigenvectors are 
\begin{align*}
\bs{n}_1(A_{\cons,k}^{\good}) & = \left(
\begin{array}{c}
(1+\frac{1}{\sqrt{1-\rho}})\bs{1} \\
\bs{1} 
\end{array}
\right), \\
\bs{n}_{n_k}(A_{\cons,k}^{\good}) & = \left(
\begin{array}{c}
(1-\frac{1}{\sqrt{1-\rho}})\bs{1} \\
\bs{1}
\end{array}
\right).
\end{align*}
which ends the proof. 

\begin{figure*}
\includegraphics[width=\textwidth]{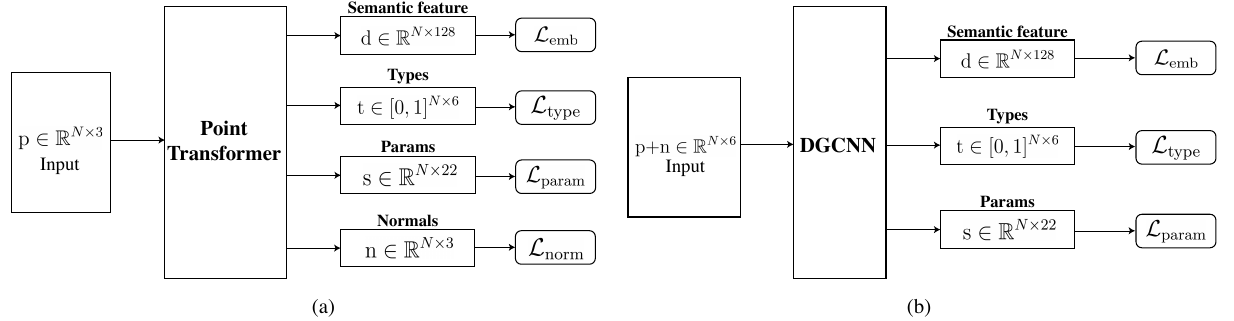}
\caption{Network architecture of Dense Descriptor Module. (a). With only point position as input. (b). With point position and normal as input.}
\label{Figure:arch1}
\vspace{-0.1in}
\end{figure*}

\subsection{Geometric Consistency Matrix Details}
Here, we describe our approach for computing the distance metric $d(p_i,\bs{s}_j)$ efficiently. 

Firstly, Dense Descriptor Module predicts three dense point-wise attributes, including a semantic feature descriptor $\bs{d} \in \realnum^{N \times 128}$, a binary type indicator vector $\bs{t} \in \{0,1\}^{N \times 6}$, and a shape parameter vector $\bs{s} \in \realnum^{N \times 22}$, where $N$ is the number of points. Then we process each primitive type $t$ respectively. If primitive type $t \in \{\plane,\sphere,\cone,\cylinder\}$, we extract the points belonging to this type according to the binary type indicator. Let $M$ be the number of points from this primitive type. Take $\plane$ as an example, we can get the corresponding shape parameter vector $s \in \realnum^{M \times 4}$. If primitive type $t \in \{\bsplineo,\bsplinec\}$, we first extract the points and take them as input to the SplineNet~\cite{SharmaLMKCM20} to get the control points of B-spline patch. Then we can compute a sub-distance matrix $d' \in \realnum^{N \times M}$, where $d'_{ij} = d(p_i,\bs{s}_j)$. Therefore, for each shape, we only need 6 iterations for each primitive type which is feasible in practice.

When computing the distance between a point and a Bspline patch, we first randomly sample each Bspline patch (1024 points), the samples are reused for all the other points. For nearest neighbor query, we used a grid data structure.

\subsection{Architecture Details of Dense Descriptor Module}
Dense Descriptor Module takes a point cloud $\set{P} = \{p_i|1\leq i \leq n\}$ as input. Each point $p_i$ has a position $\bs{p}_i\in \realnum^3$ and an optional normal $\bs{n}_i\in \realnum^3$. As illustrated in Figure~\ref{Figure:arch1}(a), with only point position as input, The dense descriptor module uses Point Transformer~\cite{zhao2020point} as backbone, and outputs four dense point-wise attributes. The attributes associated with each point $p_i\in \set{P}$ includes a semantic feature descriptor $\bs{d}_i\in \realnum^{128}$, a binary type indicator vector $\bs{t}_i\in \{0,1\}^6$, a shape parameter vector $\bs{s}_i\in \realnum^{22}$, and the point normal $\bs{n}_i\in \realnum^{3}$.

As illustrated in Figure~\ref{Figure:arch1}(b), when adding normal as input, the dense descriptor module replaces point transformer with DGCNN~\cite{wang2019dynamic}. In our experiments, we found that it has a strong ability to capture feature information of surface normal. Note that this module outputs three dense point-wise attributes.

\begin{figure*}
\centering
\footnotesize

\def\imw{0.15\textwidth}
\newcommand{\TT}[1]{\raisebox{-0.5\height}{#1}}
\setlength{\tabcolsep}{1pt}
\resizebox{0.95\textwidth}{!}{%
\begin{tabular}{cccccccc}

\rotatebox[origin=c]{90}{G.T} & 
\TT{\includegraphics[width=\imw]   {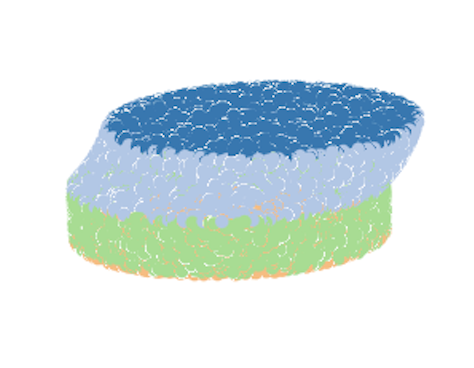}} & 
\TT{\includegraphics[height=0.11\textwidth]      {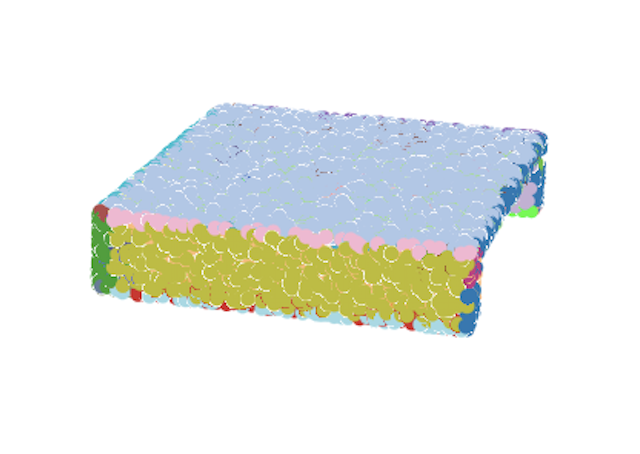}} & 
\TT{\includegraphics[width=0.16\textwidth]    {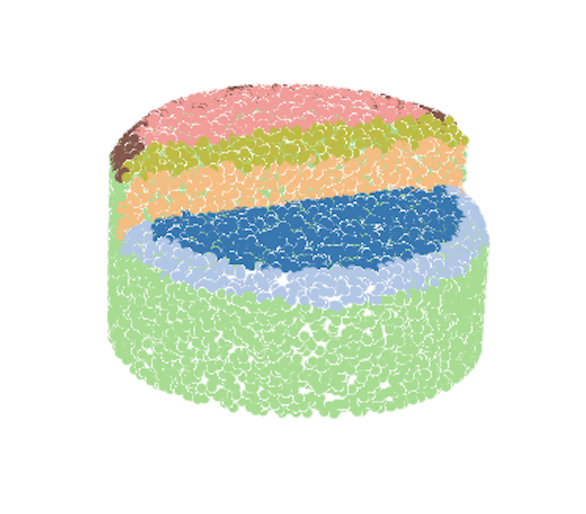}} & 
\TT{\includegraphics[width=0.12\textwidth]    {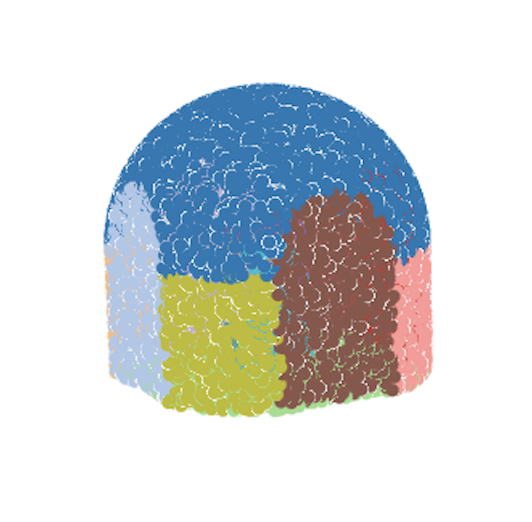}} & 
\TT{\includegraphics[width=0.13\textwidth]      {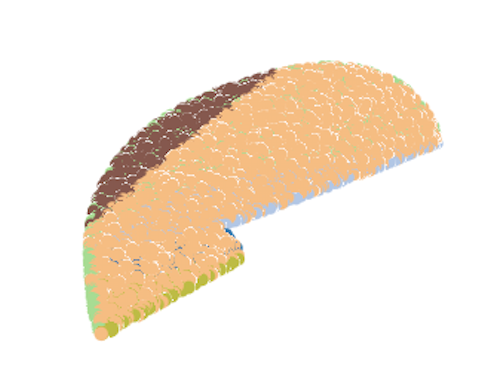}} & 
\TT{\includegraphics[width=0.13\textwidth]      {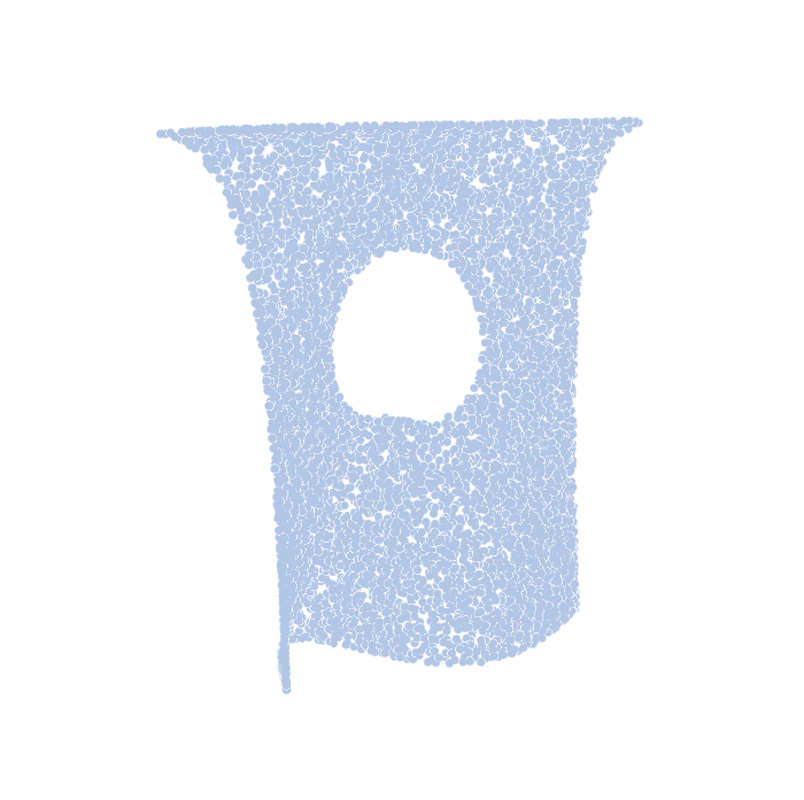}} & 
\TT{\includegraphics[width=\imw]     {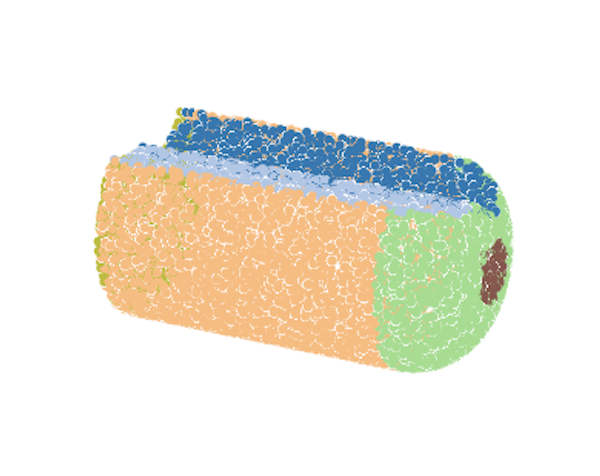}} \\

\rotatebox[origin=c]{90}{Ours-nc} & 
\TT{\includegraphics[width=\imw]   {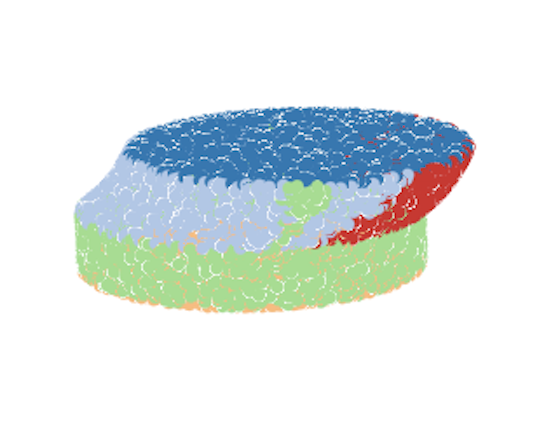}} & 
\TT{\includegraphics[height=0.11\textwidth]      {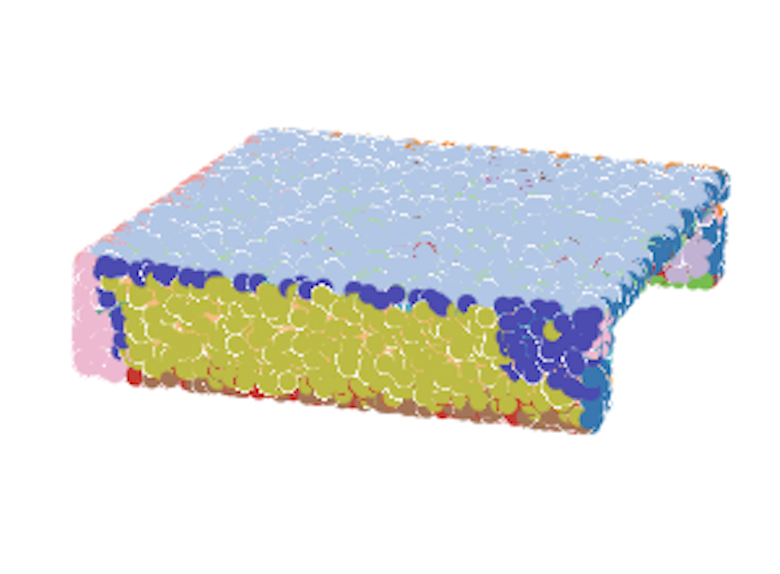}} & 
\TT{\includegraphics[width=0.14\textwidth]    {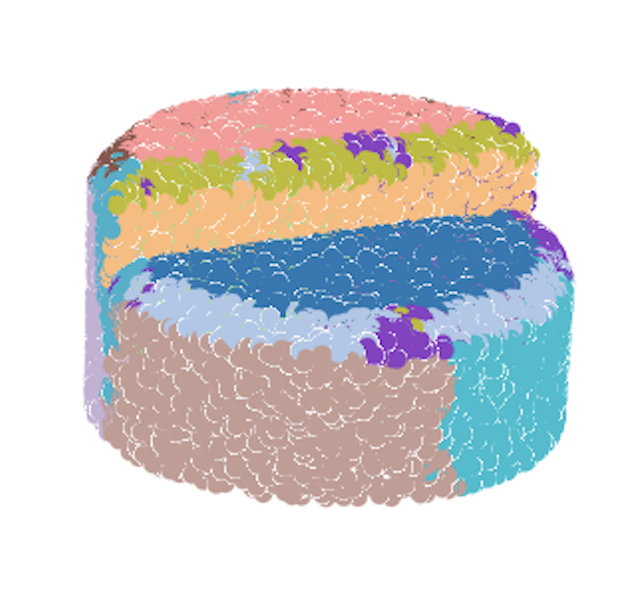}} & 
\TT{\includegraphics[width=0.12\textwidth]    {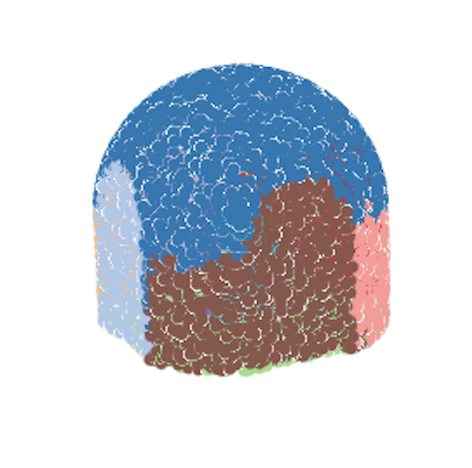}} & 
\TT{\includegraphics[width=0.13\textwidth]      {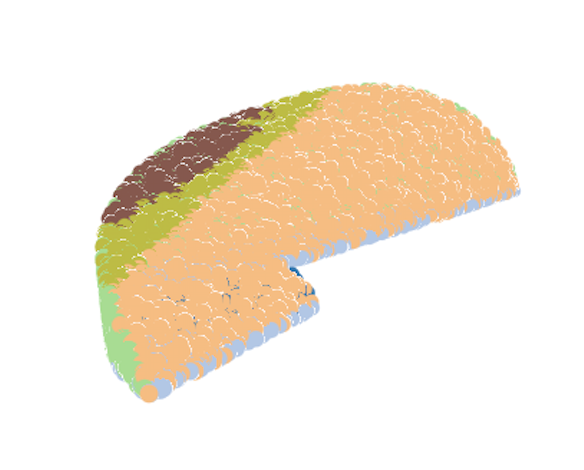}} & 
\TT{\includegraphics[width=0.13\textwidth]      {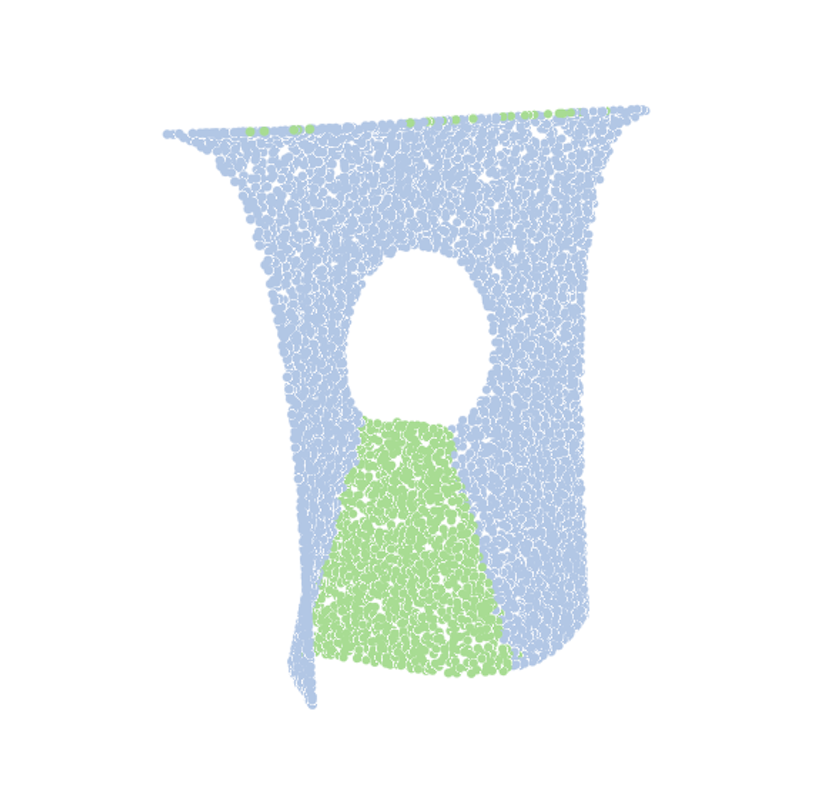}} &
\TT{\includegraphics[width=\imw]     {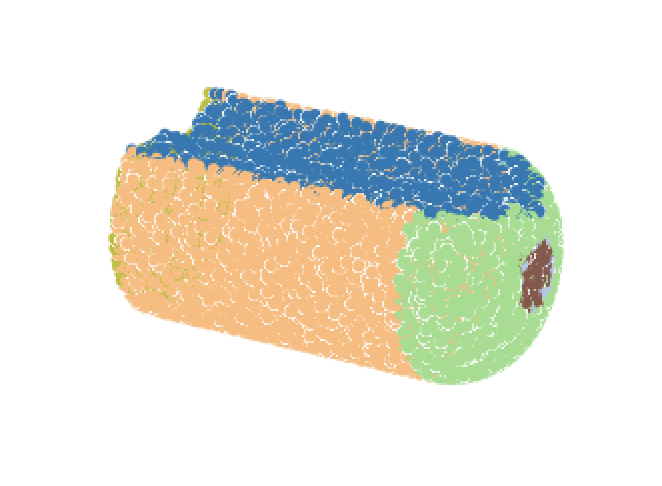}} \\

\rotatebox[origin=c]{90}{Ours-full} & 
\TT{\includegraphics[width=\imw]   {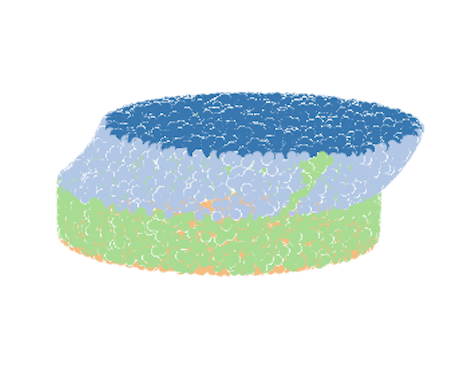}} & 
\TT{\includegraphics[height=0.11\textwidth]      {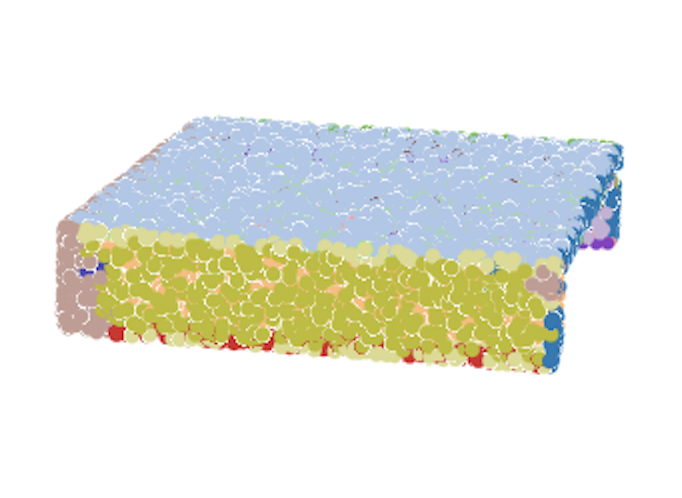}} & 
\TT{\includegraphics[width=0.145\textwidth]    {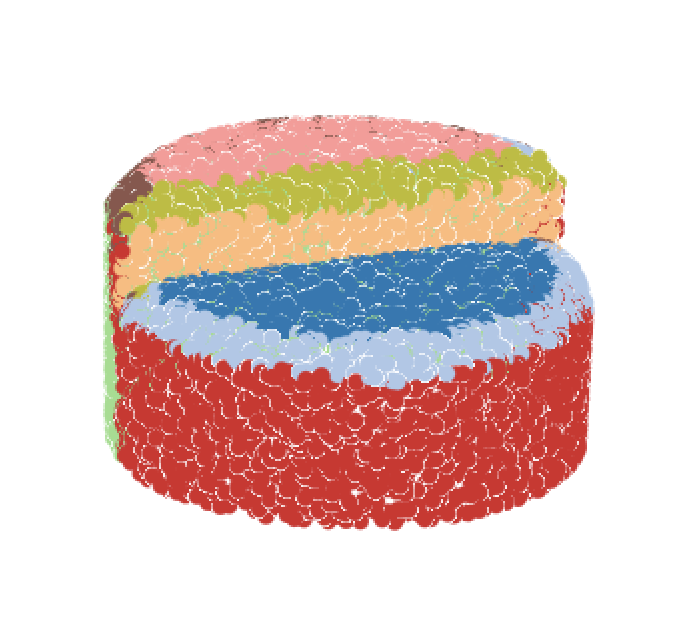}} & 
\TT{\includegraphics[width=0.12\textwidth]    {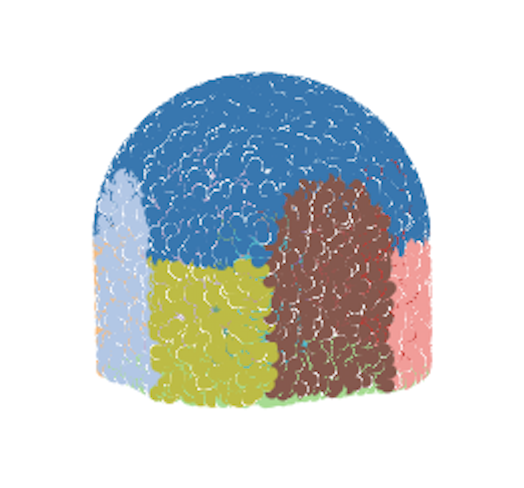}} & 
\TT{\includegraphics[width=0.13\textwidth]      {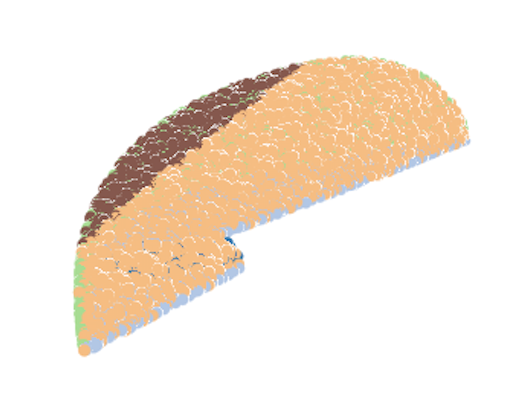}} & 
\TT{\includegraphics[width=0.13\textwidth]      {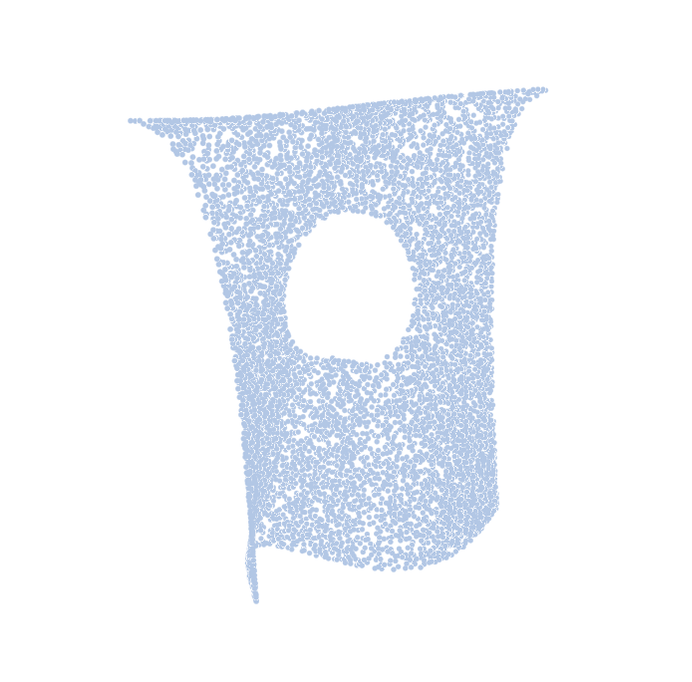}} &
\TT{\includegraphics[width=\imw]     {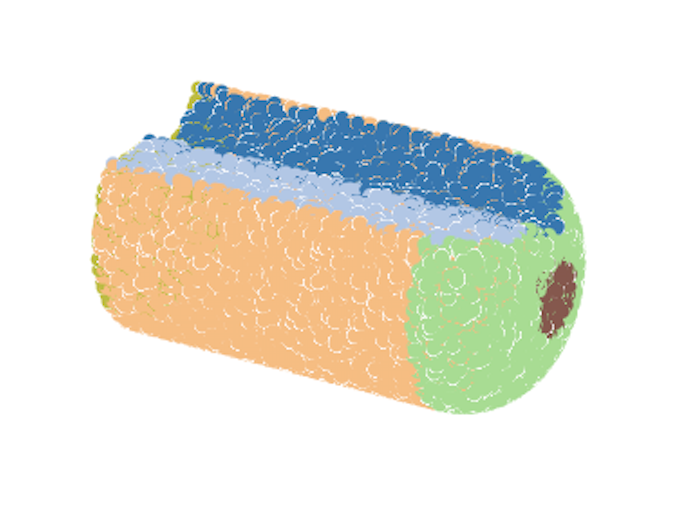}} \\

\end{tabular}
}
\caption{Comparison between our approach without combining the consistency spectral descriptors(`Ours-nc') and our full approach (`Ours-full').}
\label{Figure:Comparison_cc}
\vspace{-0.15in}
\end{figure*}

\begin{figure*}
\centering
\footnotesize

\def\imw{0.15\textwidth}
\newcommand{\TT}[1]{\raisebox{-0.5\height}{#1}}
\setlength{\tabcolsep}{1pt}
\begin{tabular}{cccccccc}

\rotatebox[origin=c]{90}{G.T} & 
\TT{\includegraphics[width=\imw]     {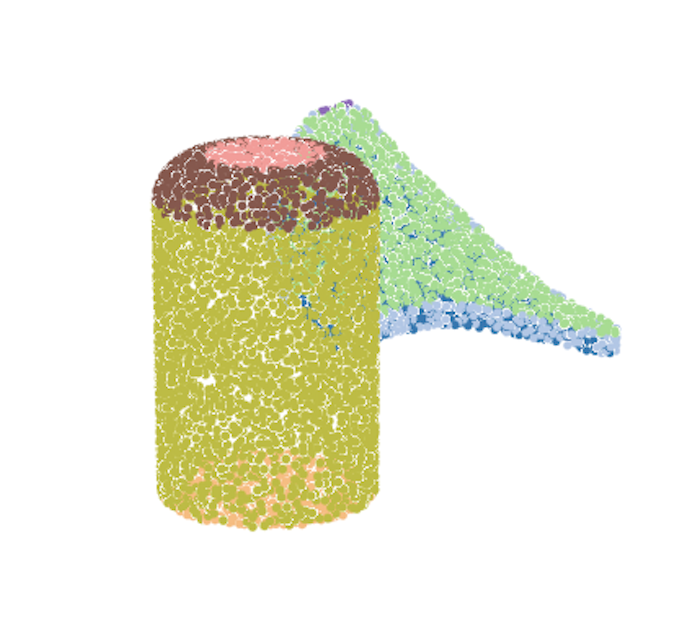}} & 
\TT{\includegraphics[width=\imw]   {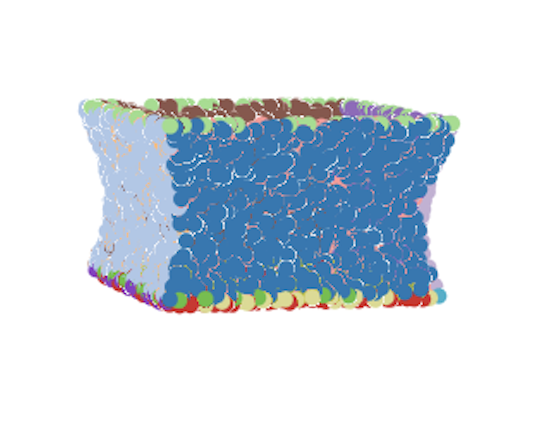}} & 
\TT{\includegraphics[height=0.15\textwidth]      {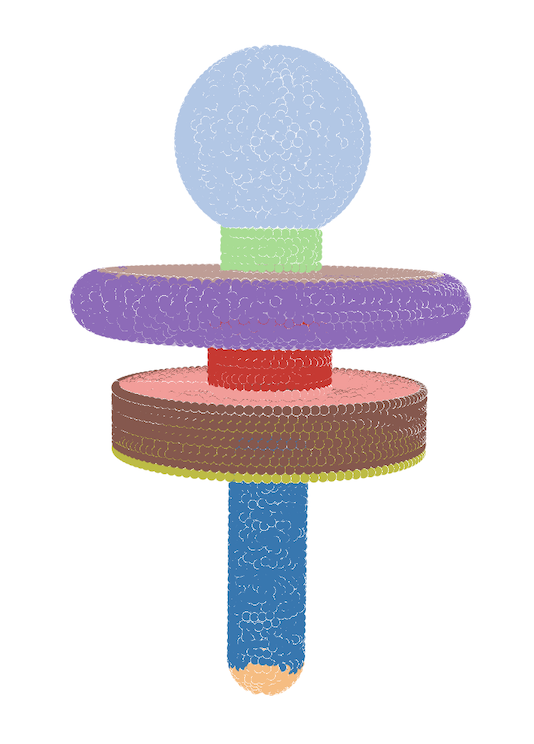}} & 
\TT{\includegraphics[width=0.12\textwidth]    {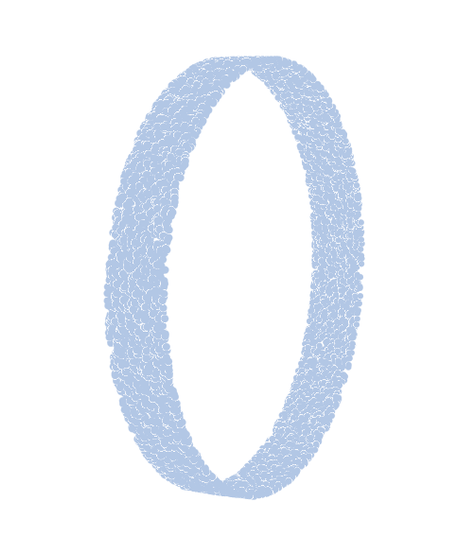}} & 
\TT{\includegraphics[width=0.09\textwidth]    {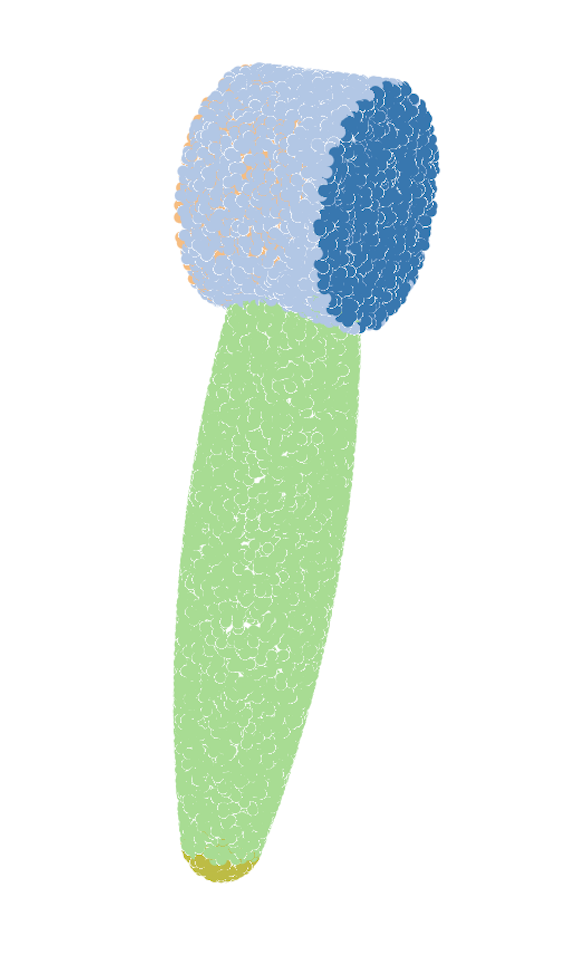}} & 
\TT{\includegraphics[width=0.13\textwidth]      {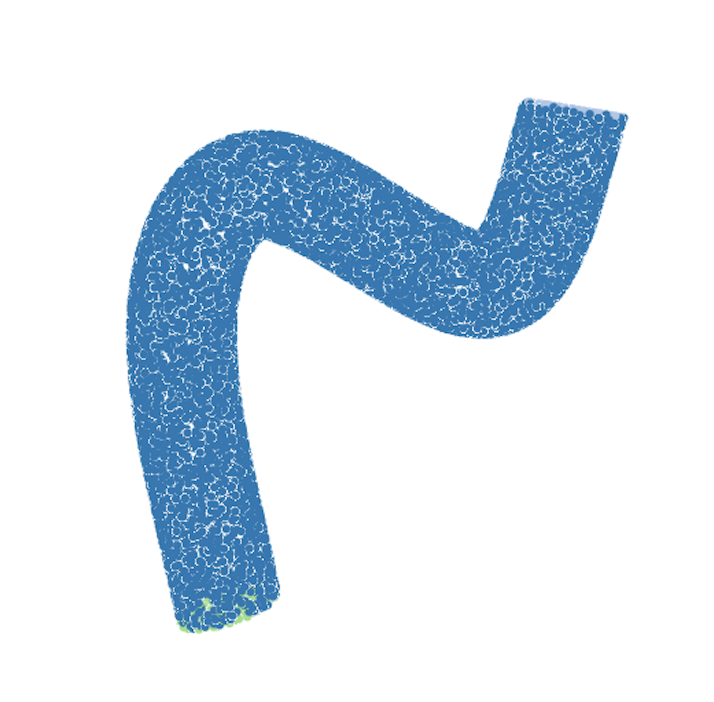}} & 
\TT{\includegraphics[width=0.14\textwidth]      {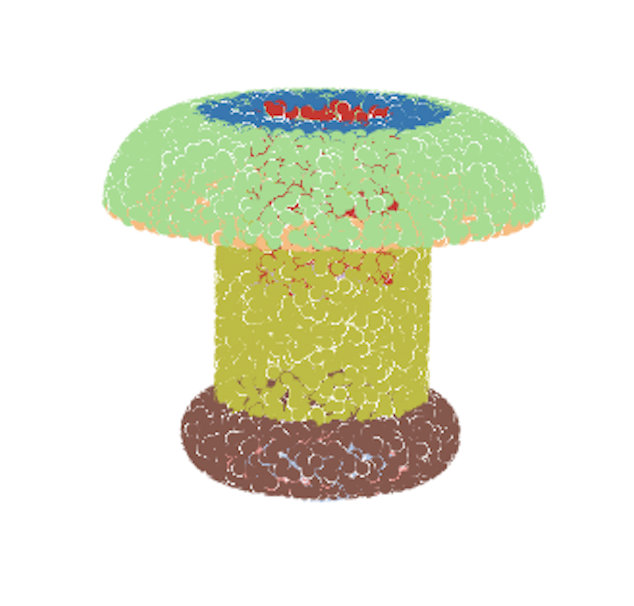}}  \\

\rotatebox[origin=c]{90}{Ours-ns} & 
\TT{\includegraphics[width=\imw]     {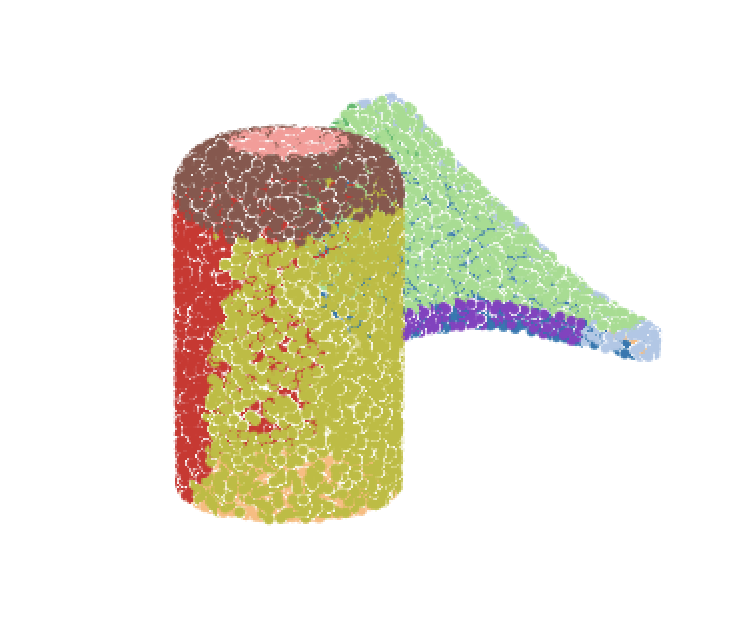}} & 
\TT{\includegraphics[width=\imw]   {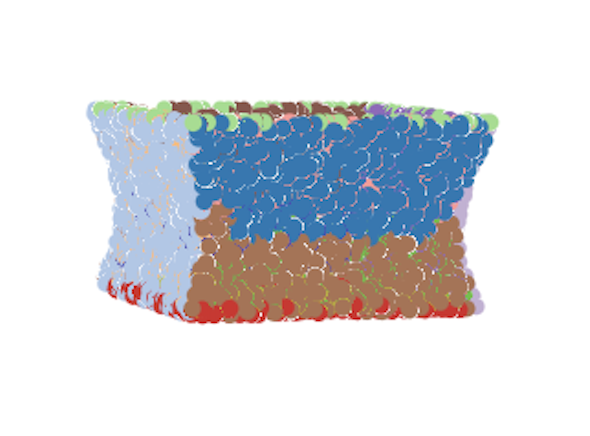}} & 
\TT{\includegraphics[height=0.15\textwidth]      {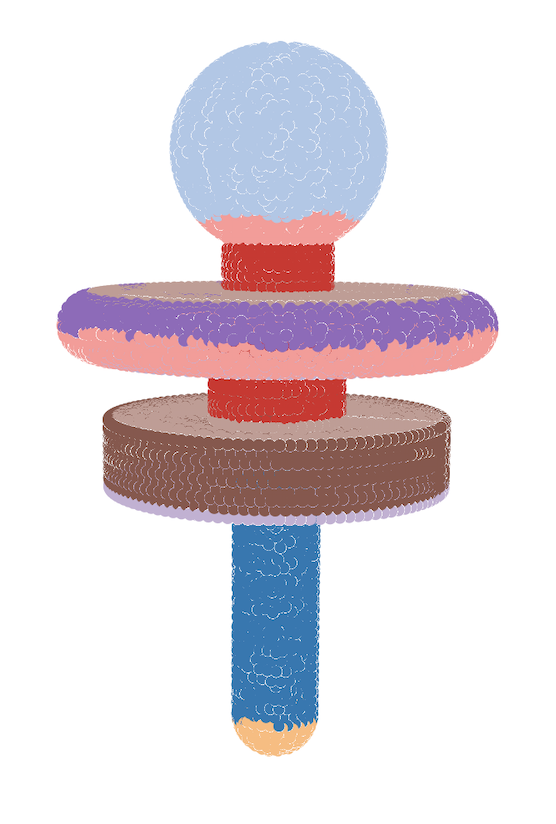}} & 
\TT{\includegraphics[width=0.10\textwidth]    {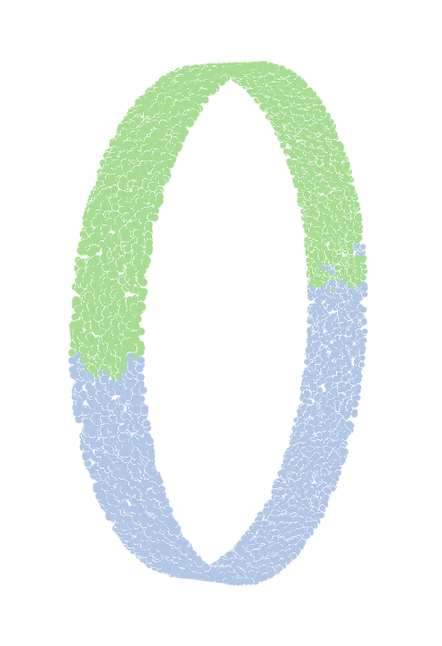}} & 
\TT{\includegraphics[width=0.085\textwidth]    {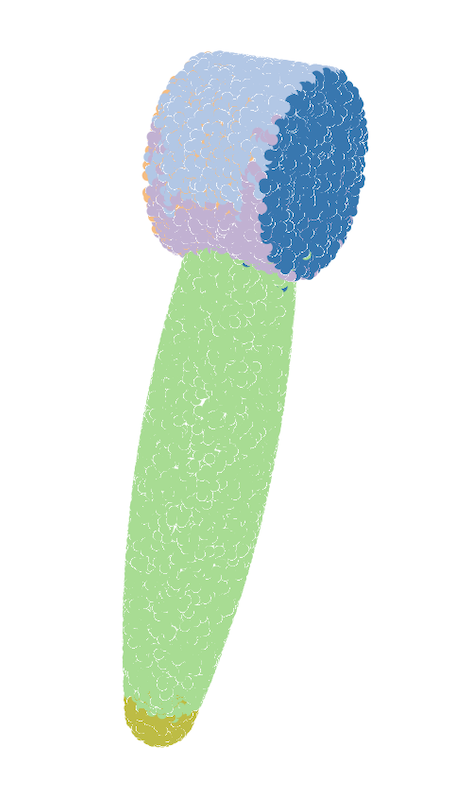}} & 
\TT{\includegraphics[width=0.14\textwidth]      {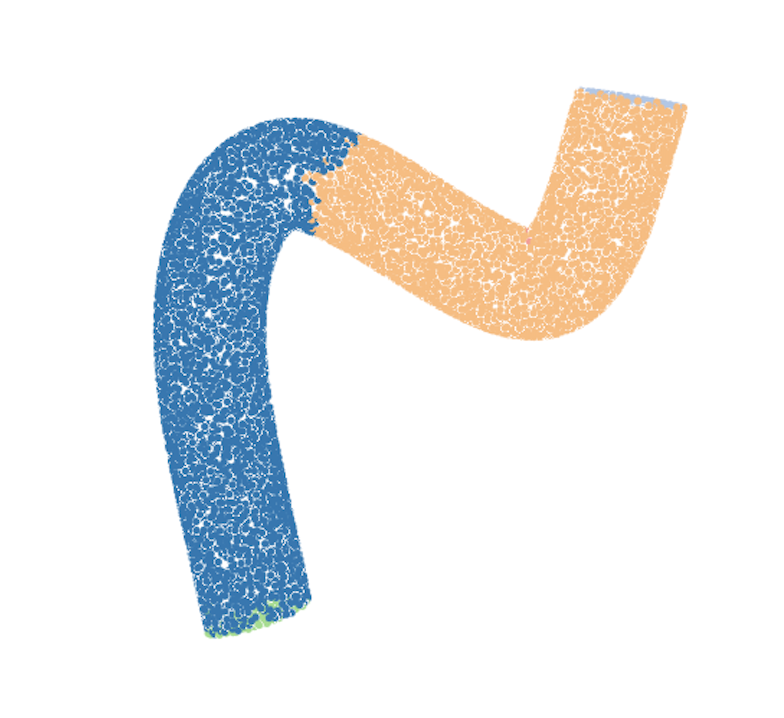}} & 
\TT{\includegraphics[width=0.15\textwidth]      {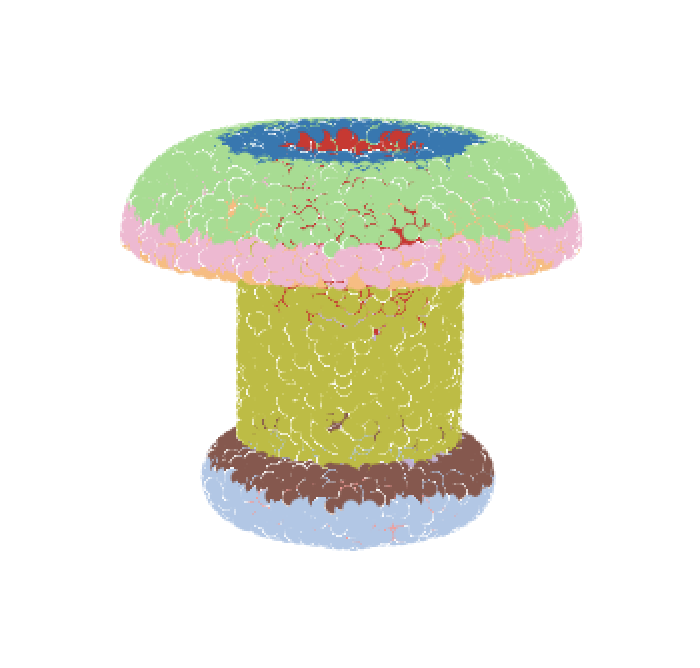}}  \\

\rotatebox[origin=c]{90}{Ours-full} & 
\TT{\includegraphics[width=\imw]     {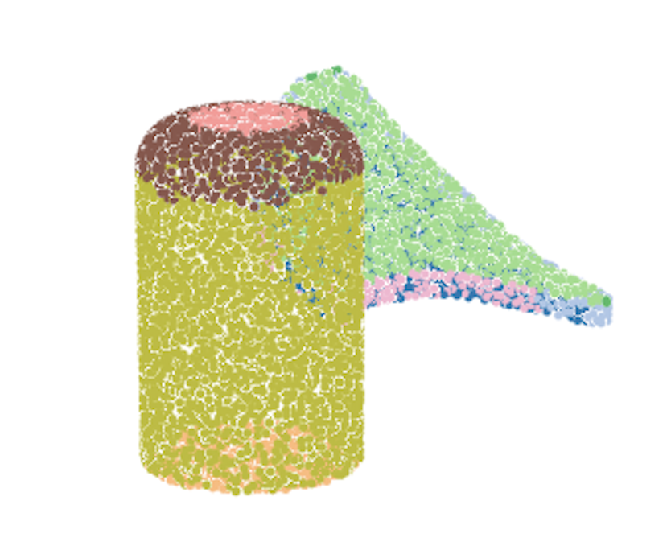}} & 
\TT{\includegraphics[width=\imw]   {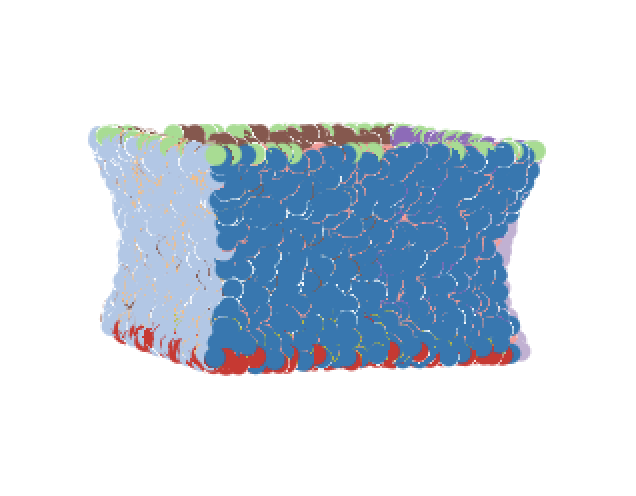}} & 
\TT{\includegraphics[height=0.15\textwidth]      {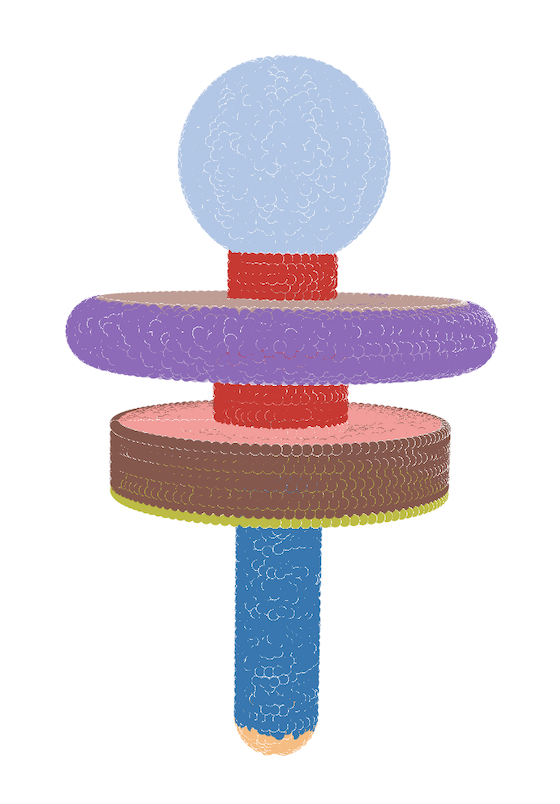}} & 
\TT{\includegraphics[width=0.12\textwidth]    {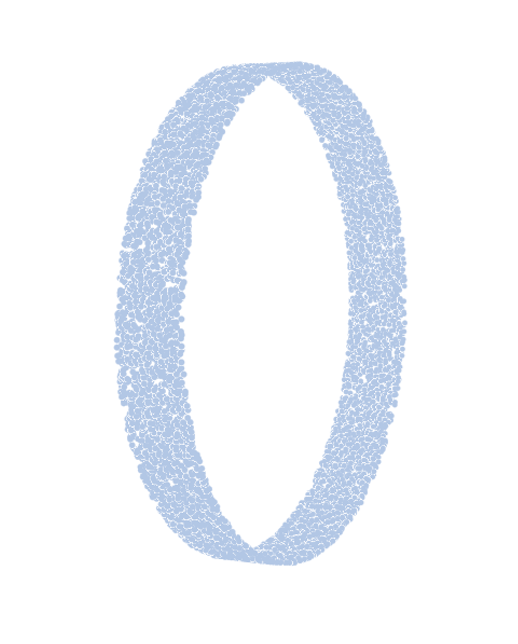}} & 
\TT{\includegraphics[width=0.09\textwidth]    {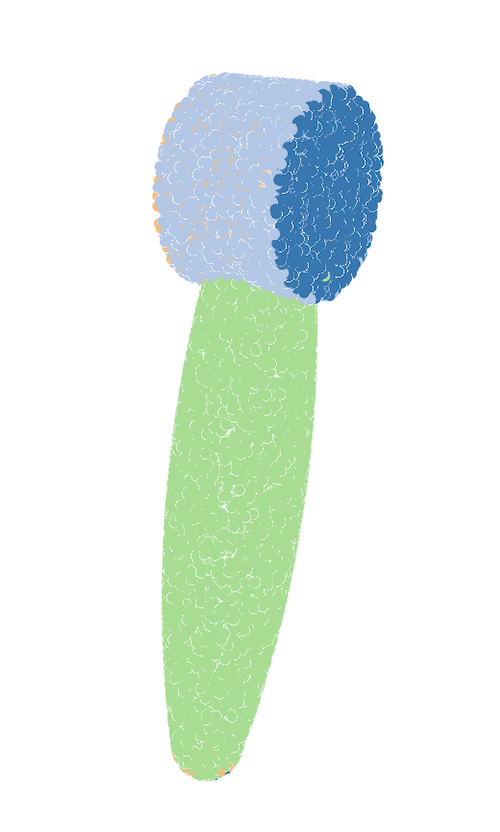}} & 
\TT{\includegraphics[width=0.13\textwidth]      {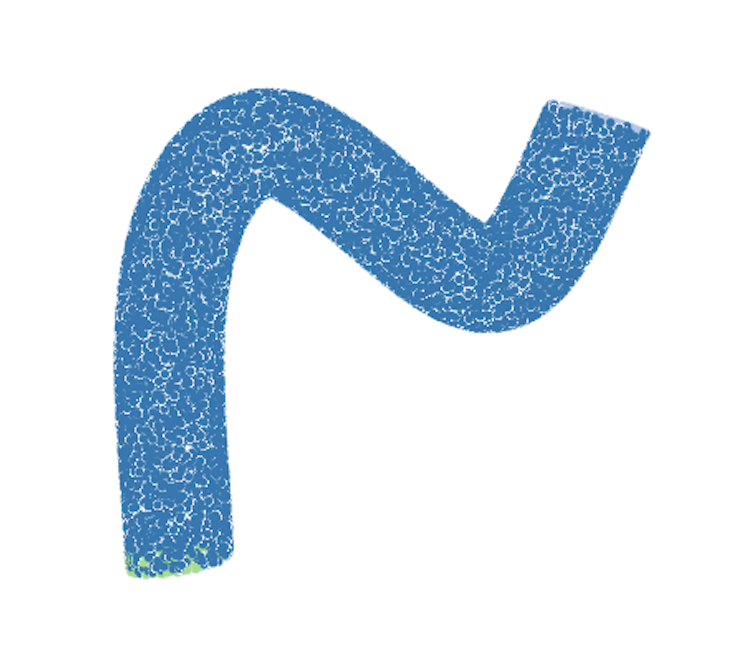}} & 
\TT{\includegraphics[width=0.14\textwidth]      {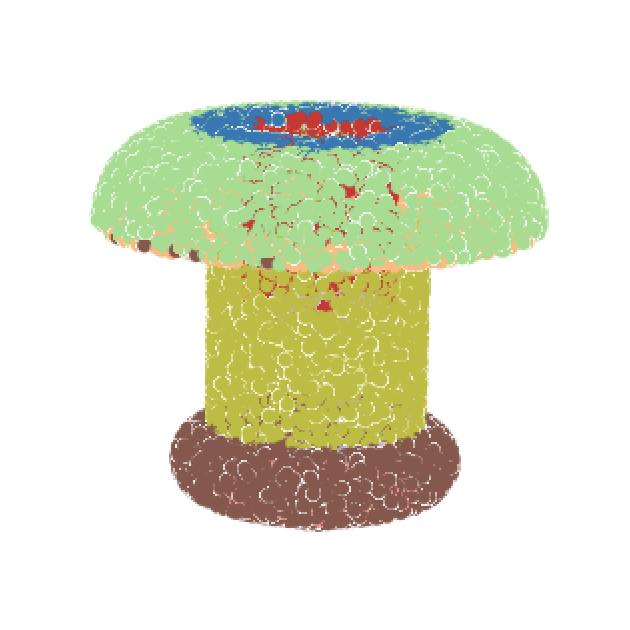}}  \\

\end{tabular}
\caption{Comparison between our approach without combining the smoothness spectral descriptors(`Ours-ns') and our full approach (`Ours-full').}
\label{Figure:Comparison_cs}
\vspace{-0.15in}
\end{figure*}

\subsection{Training Details}
\paragraph{Dataset.}
The ANSI Mechanical Component Dataset~\cite{li2019supervised} is provided by TraceParts. Four basic primitive types (plane, sphere, cylinder, cone) cover 94\% percentage area per-model on average in ANSI. The maximum
number of primitives per shape does not exceed 20 in all the models. In experiments, we first uniformly sample 8192 points over the entire surface of each shape as the input point cloud . Then we normalize each shape so that its mean is at the origin, and the diameter of the shape is 1. During training, we perturb the input model by randomly moving each point along along the surface normal direction with a random value in $[-0.01, 0.01]$.

The ABCParts dataset is derived from the ABC dataset~\cite{SharmaLMKCM20}. Each model consists of at least one B-spline patch. In the experiments, we first sample each shape with 10K points randomly distributed
on the shape surface as the input point cloud. Similar to ANSI, during training, we also randomly perturb each data point along the surface normal direction in $[-0.01, 0.01]$ range. The normals are also perturbed with random noise in a uniform range of $[-3, 3]$ degrees from their original direction. All the baseline approaches share the same data preprocessing procedure with our method.

\paragraph{Training Procedure Details.}
Network training of HPNet consists of two stages. The first stage learns the Dense Descriptor Module. Without normal as input, we use default hyperparameters of network with batch size 32, initial learning rate $1 \times 10^{-2}$. Learning rate reduces by the factor of 10 when the validation performance convergence. The experiment took 20 hours on a Tesla V100 GPU. With normal as input, we use default hyperparameters of network with batch size 8, initial learning rate $1 \times 10^{-3}$. Learning rate reduces by the factor of 2 when the validation performance converges. The experiment on each dataset took 50 hours on a Tesla V100 GPU.

\subsection{Visualization of Different Feature Combinations}
Here, we show more visualization results to continue to study the impacts of different components of HPNet.

Figure~\ref{Figure:Comparison_cc} shows qualitative results for comparisons between our approach without the consistency spectral descriptors and our full approach. When the model shows accurate predictions of primitive parameters, combining geometry consistency spectral descriptor can segment the primitive patch more precisely (columns 2 and 4). This is because of the points from the same primitive share nearly the same primitive parameters. In this case, the geometry consistency descriptor can also help merge two patches that belong to the same primitive into one patch (columns 1, 3, and 6). Moreover, when two different primitive patches are erroneously merged, it can help separate them (columns 4 and 7). 

Figure~\ref{Figure:Comparison_cs} shows more results that compare our approach without the smoothness spectral descriptors with our full approach. Besides capturing sharp edges between different primitives, the smoothness spectral descriptor can also help rectify two patches when their boundaries are smooth.
