# Supplementary material for: HPNet: Deep Primitive Segmentation Using Hybrid Representations
Source: arXiv:2105.10620 source file (2021-10-21)
Supplement: Supplementary file 3 [file supp_figure4.tex]

\begin{figure*}
\centering
\footnotesize

\def\imw{0.15\textwidth}
\newcommand{\TT}[1]{\raisebox{-0.5\height}{#1}}
\setlength{\tabcolsep}{1pt}
\begin{tabular}{cccccccc}

\rotatebox[origin=c]{90}{G.T} & 
\TT{\includegraphics[width=\imw]     {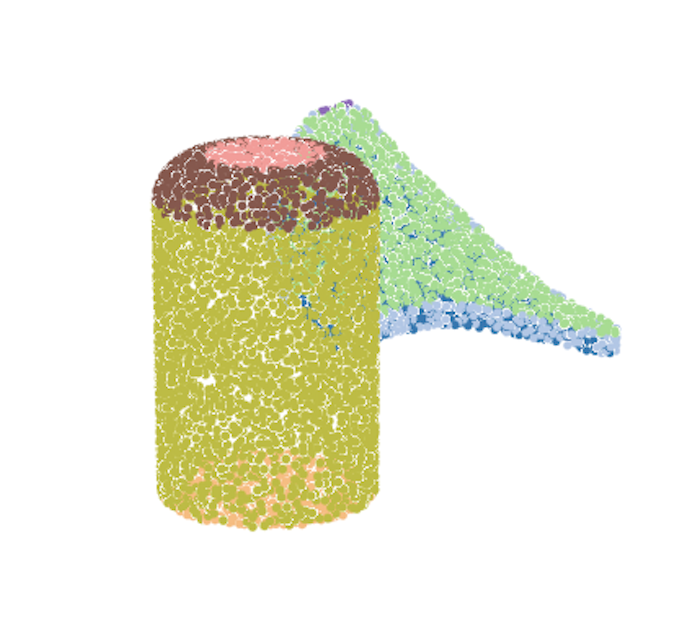}} & 
\TT{\includegraphics[width=\imw]   {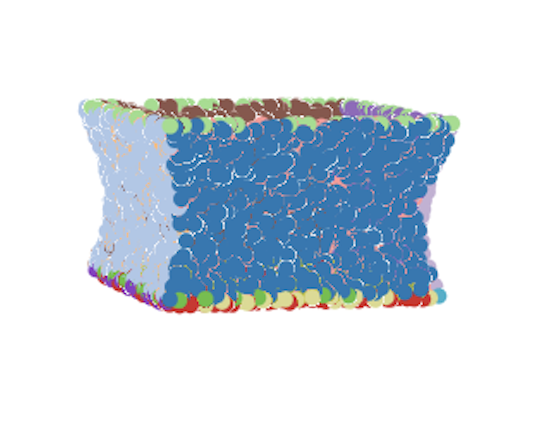}} & 
\TT{\includegraphics[height=0.15\textwidth]      {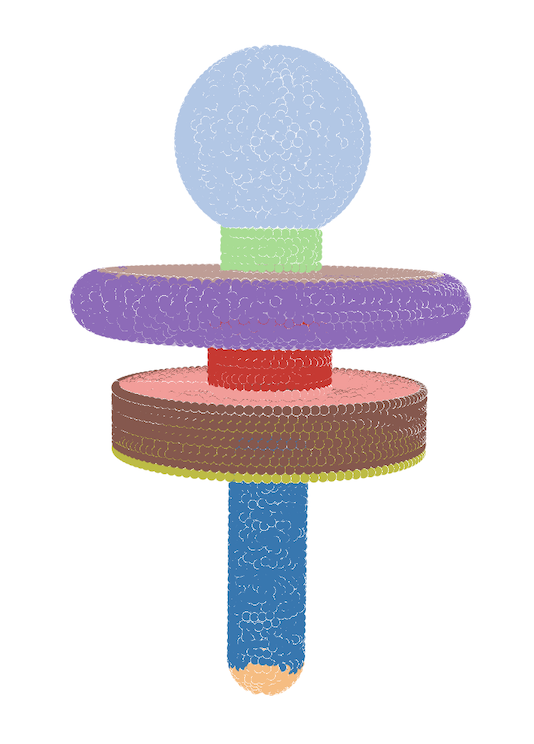}} & 
\TT{\includegraphics[width=0.12\textwidth]    {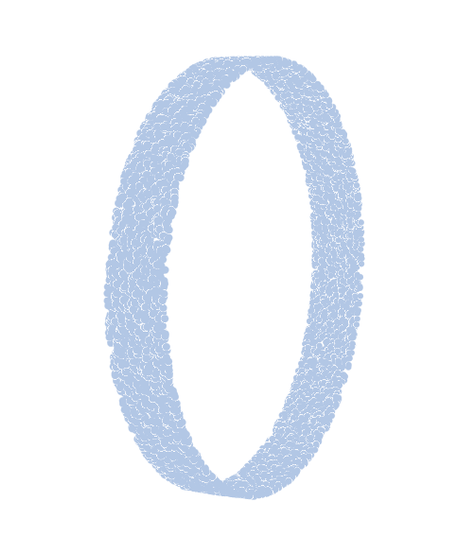}} & 
\TT{\includegraphics[width=0.09\textwidth]    {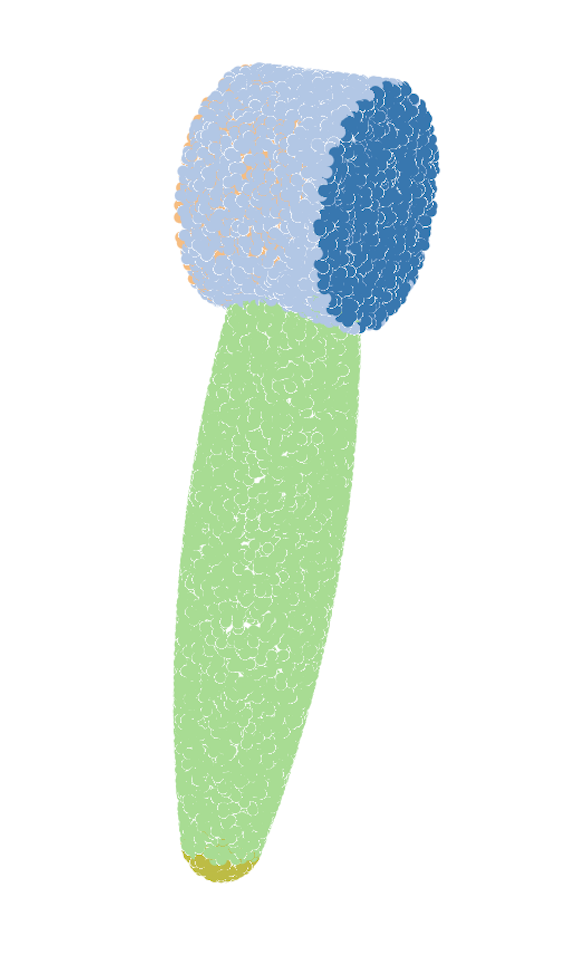}} & 
\TT{\includegraphics[width=0.13\textwidth]      {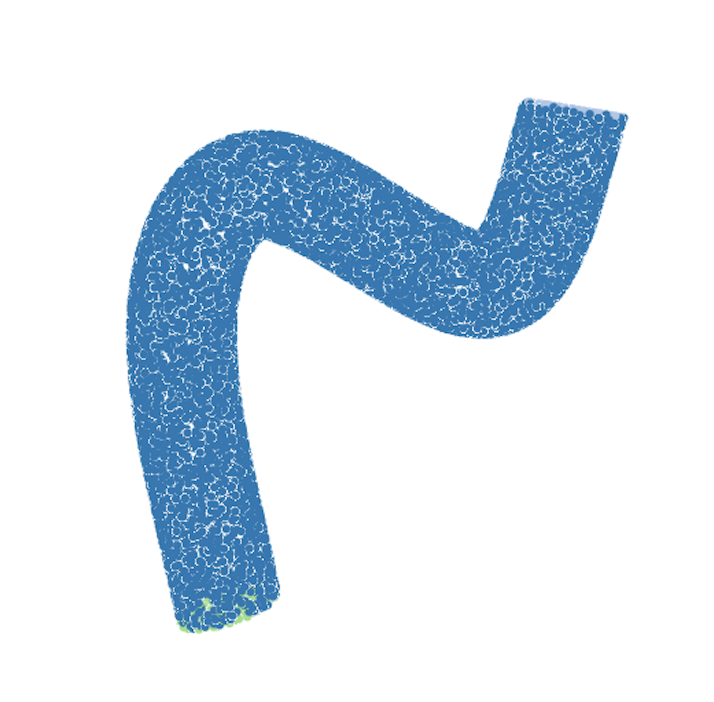}} & 
\TT{\includegraphics[width=0.14\textwidth]      {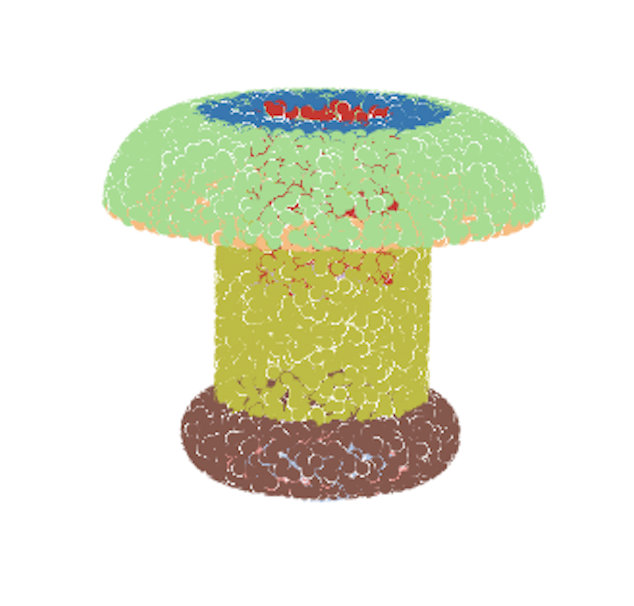}}  \\

\rotatebox[origin=c]{90}{Ours-ns} & 
\TT{\includegraphics[width=\imw]     {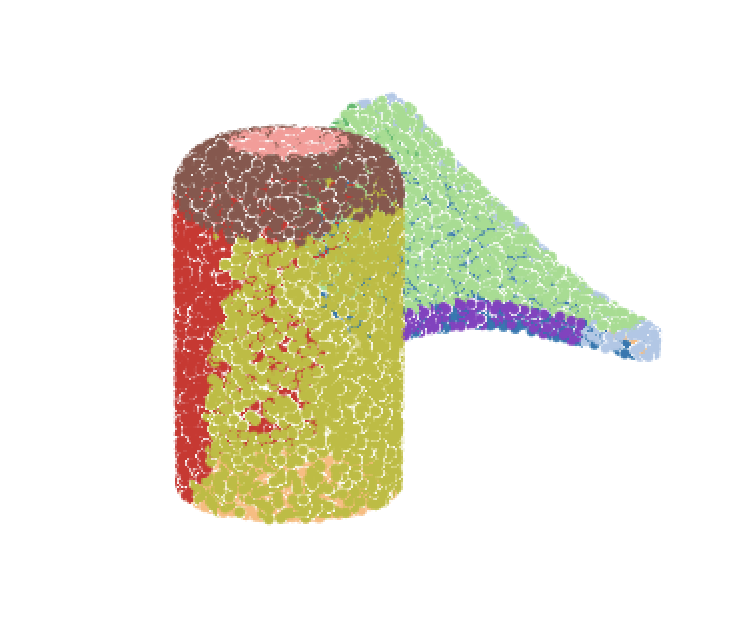}} & 
\TT{\includegraphics[width=\imw]   {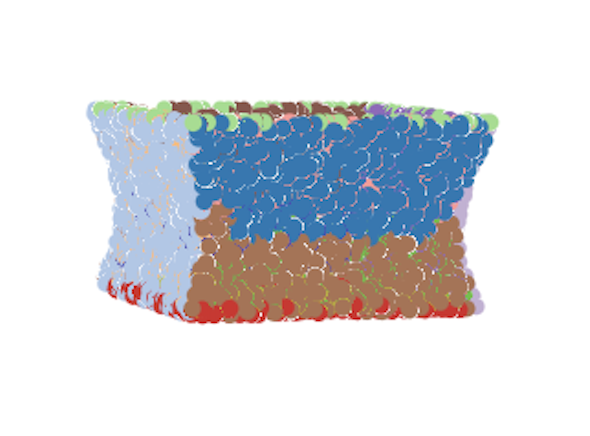}} & 
\TT{\includegraphics[height=0.15\textwidth]      {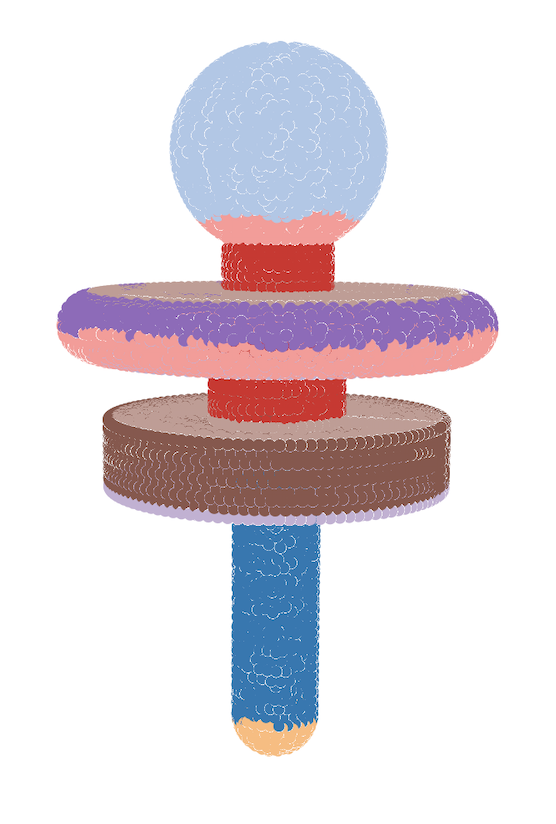}} & 
\TT{\includegraphics[width=0.10\textwidth]    {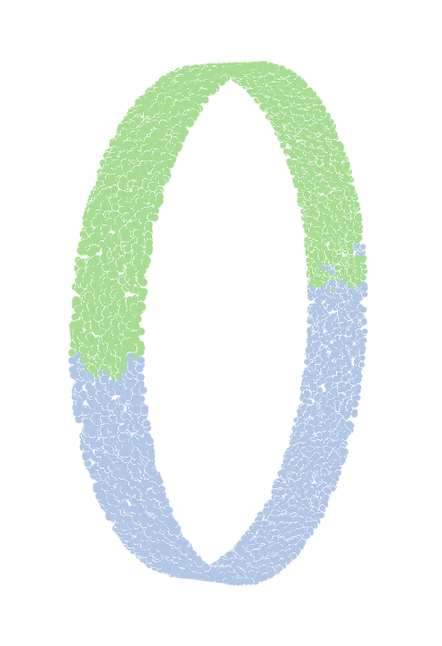}} & 
\TT{\includegraphics[width=0.085\textwidth]    {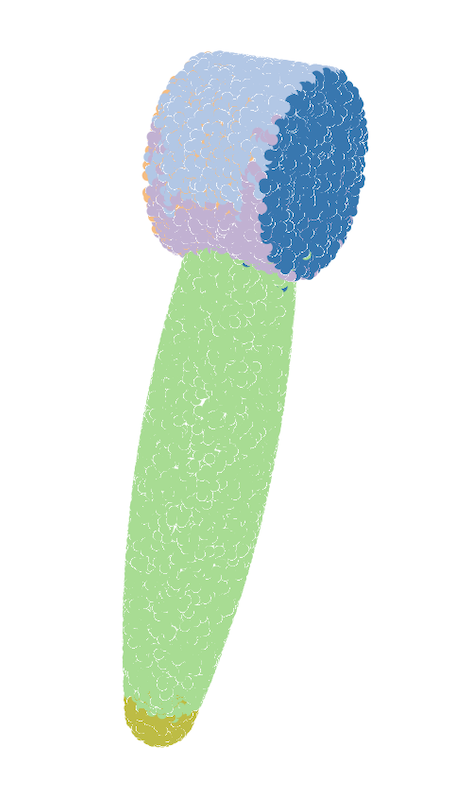}} & 
\TT{\includegraphics[width=0.14\textwidth]      {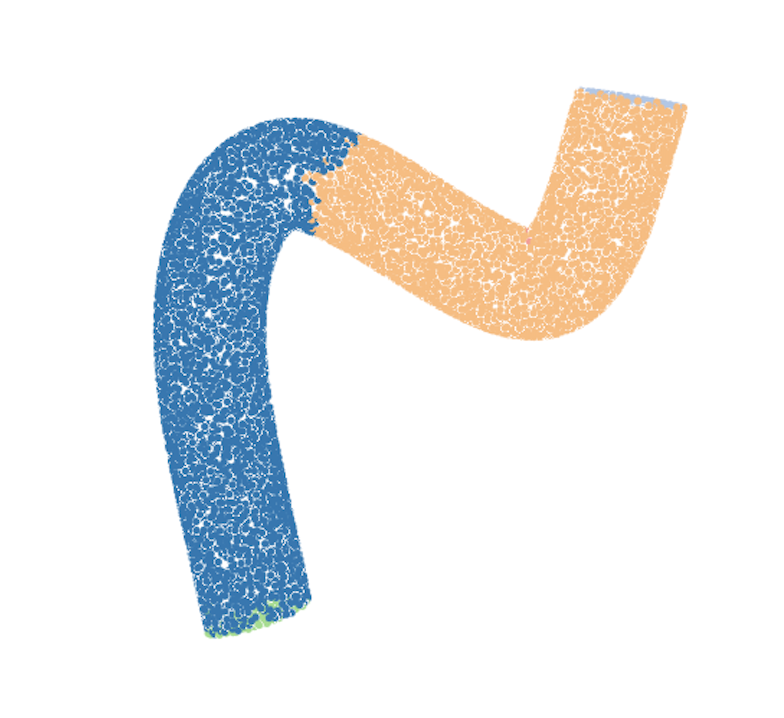}} & 
\TT{\includegraphics[width=0.15\textwidth]      {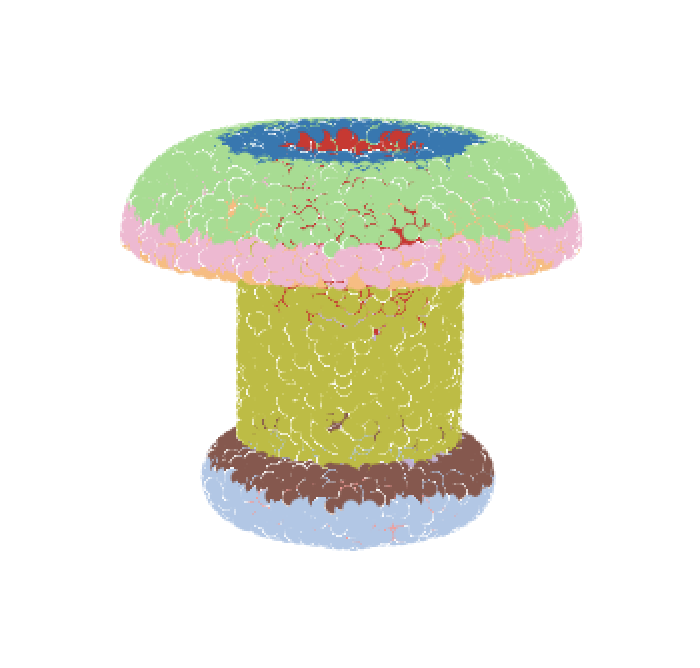}}  \\

\rotatebox[origin=c]{90}{Ours-full} & 
\TT{\includegraphics[width=\imw]     {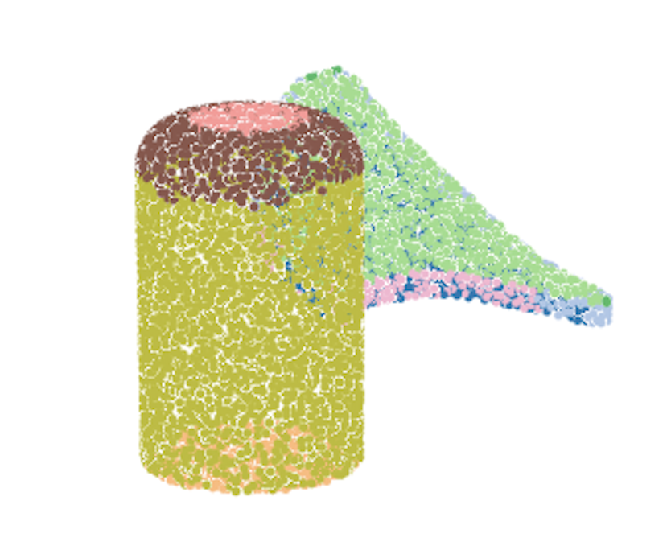}} & 
\TT{\includegraphics[width=\imw]   {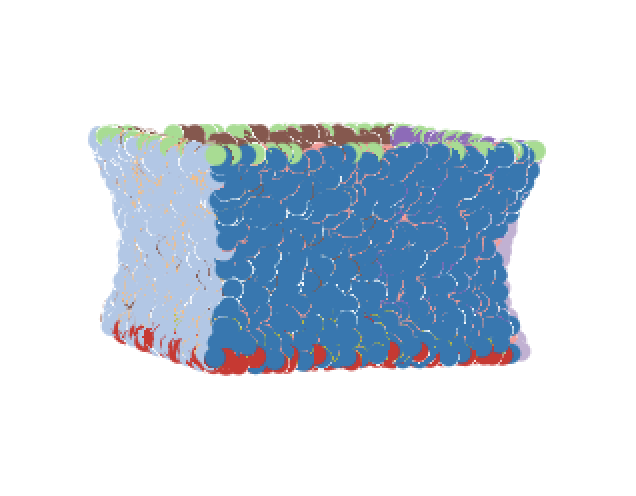}} & 
\TT{\includegraphics[height=0.15\textwidth]      {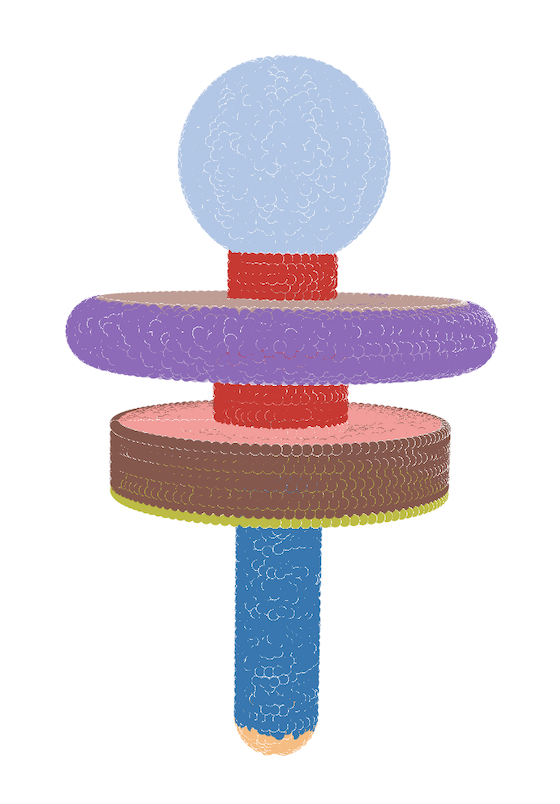}} & 
\TT{\includegraphics[width=0.12\textwidth]    {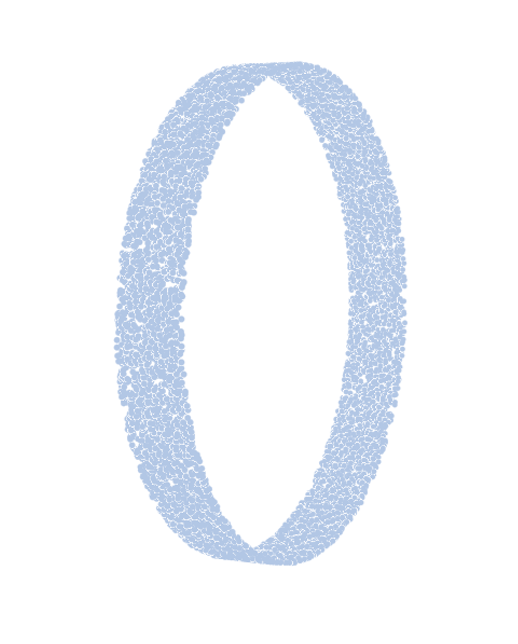}} & 
\TT{\includegraphics[width=0.09\textwidth]    {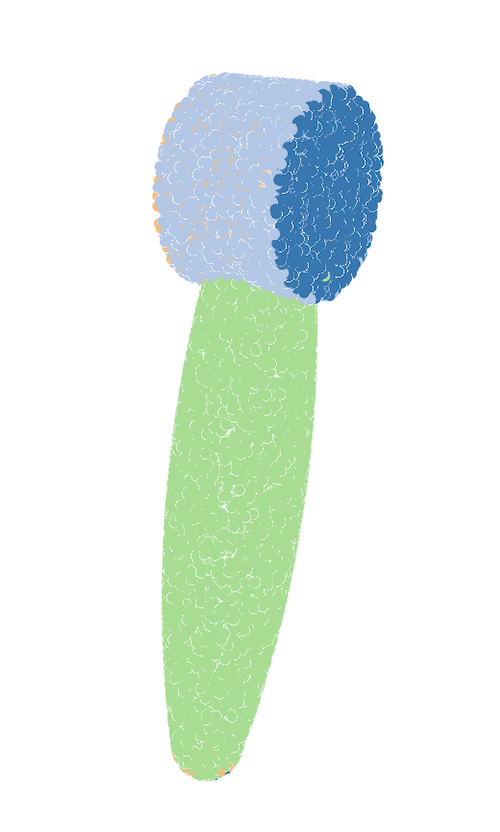}} & 
\TT{\includegraphics[width=0.13\textwidth]      {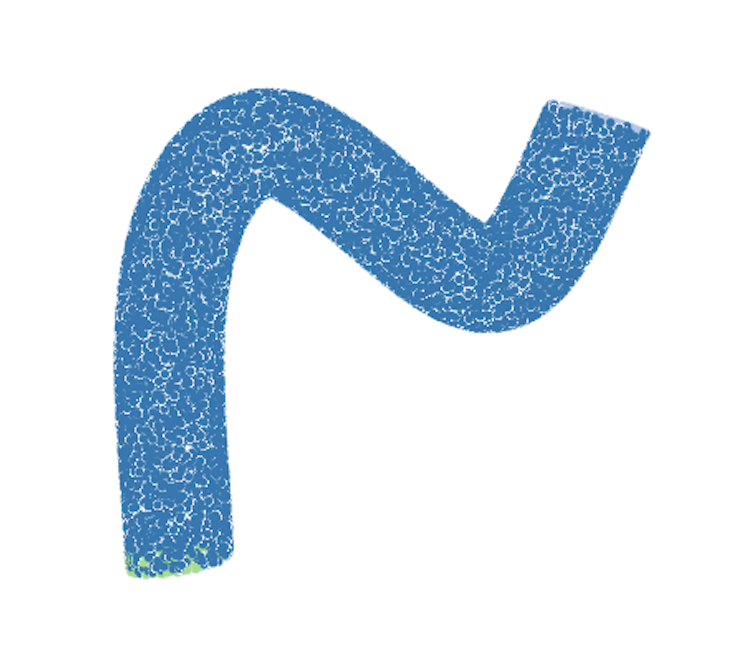}} & 
\TT{\includegraphics[width=0.14\textwidth]      {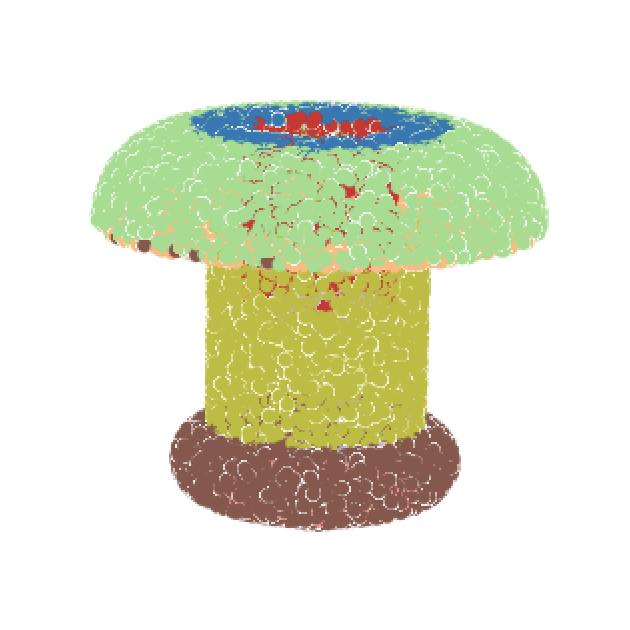}}  \\

\end{tabular}
\caption{Comparison between our approach without combining the smoothness spectral descriptors(`Ours-ns') and our full approach (`Ours-full').}
\label{Figure:Comparison_cs}
\vspace{-0.15in}
\end{figure*}
